# Supplementary material for: Bayesian Decision Trees via Tractable Priors and Probabilistic Context-Free Grammars
Source: arXiv:2302.07407 source file (2023-02-15)
Supplement: Supplementary file 1 [file 9-Appendix1.tex]

% !TEX root = 0-main.tex

\newpage
\appendix
\onecolumn
\section{Proofs of Theorems}

Appendix stuff
